# Supplementary material for: Cloud Feedback on Earth's Long-term Climate Simulated by a Near-global Cloud-permitting Model
Source: arXiv:2209.02519 source file (2022-09-06)
Supplement: Supplementary file 1 [file GRL_SI.pdf]

# Supporting Information for "Cloud Feedback on Earth's Long-term Climate Simulated by a Near-global Cloud-permitting Model"

Mingyu Yan[1], Jun Yang[1], Yixiao Zhang[1,2], Han Huang[1,3]

[1]Laboratory for Climate and Ocean-Atmosphere Studies, Department of Atmospheric and Oceanic Sciences, School of Physics, Peking University, Beijing 100871, China

[2]Now at Department of Earth Atmospheric and Planetary Sciences, Massachusetts Institute of Technology, 77 Massachusetts Avenue, Cambridge, MA 02139, USA

[3]Now at Department of Atmospheric and Oceanic Sciences, McGill University, Montreal, Canada

**Contents of this file**

1. Text S1. More details on experimental designs
2. Text S2. The calculation of shortwave cloud feedback
3. Text S3. Inversion strength indexes
4. Figures S1 to S12

**Text S1. More details on experimental designs**

We did seven fixed SST simulations. In these simulations, the solar radiation is 0.70, 0.75, 0.80, 0.85, 0.90, 0.95, and 1.00 $S_0$ ($S_0 = 1361.3\ \mathrm{W\,m^{-2}}$) and the corresponding $CO_2$ concentration is 366.20, 184.50, 89.26, 38.20, 14.80, 4.55, and 1.04×$CO_2$, respectively, where 1.00×$CO_2$ is 355 ppmv. We firstly run the control simulation (0.70$S_0$) for 150 model days to generate the initial fields of the other experiments. Then, we run the other experiments starting from the final state of the control simulation for 130 model days. Time series of clouds and energy balances show that each simulation reaches a quasi-equilibrium state after about 100 days (Figure S1). The last 30 days are used for the analyses.

Although there are energy imbalances induced by the fixed SST distribution, the energy budget for the atmosphere itself is balanced (Figure S1l). For example, energy imbalances (upward positive) of the TOA, the surface, and the atmosphere are respectively 33, 32, and 1 W $m^{-2}$ in the 1.00$S_0$ case. Moreover, the degrees of energy imbalance among all seven experiments are quite similar (Figure S1j).

To reduce the energy imbalances at the TOA and the surface, another four fixed SST simulations were run. The solar radiation is 0.85, 0.95, 1.05, and 1.15 $S_0$ and the corresponding $CO_2$ concentration is 366.20, 89.26, 14.80, and 1.04×$CO_2$, respectively. For these four simulations, the energy imbalances at the TOA and the surface decrease to be less than 3 $\mathrm{W\,m^{-2}}$ (Figure S3).

We also add two slab ocean tests, within which all the TOA, the atmosphere, and the surface are in energy balance. These two cases were run with a horizontal spacing of 42 km, which is coarser than that used in the fixed SST simulations, due to the high computational cost. The domain size is the same as that in the fixed SST simulations. In these two experiments, an ocean depth of 1 m is used, and planetary obliquity is 23.5°. The solar constants are 0.85 $S_0$ and 0.95 $S_0$. We have adjusted atmospheric $CO_2$ concentration to achieve a similar global-mean surface temperature between these two runs; the $CO_2$ concentrations are 152,650 ppmv for 0.85 $S_0$ and 63,900 ppmv for 0.95 $S_0$. These two simulations were run for 500 days, and the global-mean surface temperatures are 292.5 K and 292.9 K, respectively (Figure S4).

Note that the grid spacing (42 km) of the slab ocean runs is too coarse to be called cloud-permitting simulations. Nevertheless, the trends of the cloud properties (such as cloud fraction, cloud water path, cloud radiative effect, and planetary albedo) are the same as those in the fixed SST experiments.

**Text S2. The calculation of shortwave cloud feedback**

The value of shortwave cloud effect ($SWCE$) in the model is calculated as the difference between all-sky and clear-sky net shortwave fluxes at the TOA. For two solar constants of $S_1$ and $S_2$, $SWCE$ can be expressed as:

$$SWCE_1 = (\alpha_{pc}^1 - \alpha_p^1)\frac{S_1}{4}, \tag{1}$$

$$SWCE_2 = (\alpha_{pc}^2 - \alpha_p^2)\frac{S_2}{4}, \tag{2}$$

where $\alpha_{pc}$ is the clear-sky planetary albedo, and $\alpha_p$ is the all-sky planetary albedo. Note that the denominator is 4.0 for the CAM4 experiments of Goldblatt et al. (2021) but 3.87 for our SAM experiments, because SAM uses Cartesian geometry and meanwhile the polar regions are not simulated.

The change of the $SWCE$ is contributed by two parts, one is from the change of the solar radiation without any change of the cloud properties, and the other one is from the change of the cloud properties without any change of solar radiation. Combining Equations 1 and 2, one could find that:

$$\begin{aligned} SWCE_2 - SWCE_1 &= (\alpha_{pc}^2 - \alpha_p^2)\frac{S_2}{4} - (\alpha_{pc}^1 - \alpha_p^1)\frac{S_1}{4} \\ &= (\alpha_p^1 - \alpha_p^2)\frac{S_2}{4} - (\alpha_{pc}^1 - \alpha_p^1)\frac{S_1}{4} + (\alpha_{pc}^2 - \alpha_p^1)\frac{S_2}{4} \end{aligned} \tag{3}$$

In the simulations, the change of the clear-sky albedo is very small (less than 0.001 in SAM and less than 0.01 in CAM4). We can assume that $\alpha_{pc}^1$ is approximately equal to $\alpha_{pc}^2$, so that Equation 3 can be re-written as:

$$\underbrace{SWCE_2 - SWCE_1}_{\text{change of shortwave cloud radiative effect}} \approx \underbrace{(\alpha_p^1 - \alpha_p^2)\frac{S_2}{4}}_{\textbf{shortwave cloud feedback}} + \underbrace{(\alpha_{pc}^1 - \alpha_p^1)(\frac{S_2}{4} - \frac{S_1}{4})}_{\text{change of the shortwave cloud radiative effect due to the change of insolation without any change of the cloud properties}} \tag{4}$$

For example, in the two CAM4 experiments of $S_1 = 1.00S_0$ and $S_2 = 0.80S_0$ in Goldblatt et al. (2021), $\alpha_p^1$ is 0.32, $\alpha_p^2$ is 0.28, $\alpha_{pc}^1$ is 0.17, $SWCE_1$ is $-52.5$ W m$^{-2}$, $SWCE_2$ is $-33.4$ W m$^{-2}$. So, the change of the shortwave cloud radiative effect (the left-hand side of Equation 4) is 19.1 W m$^{-2}$, the first term on the right-hand side of Equation 4 is 10.9 W m$^{-2}$, and the second term is 10.2 W m$^{-2}$. In other words, in these two experiments the strength of the shortwave cloud feedback is 10.9 W m$^{-2}$ rather than 19.1 W m$^{-2}$.

Moreover, in the two SAM experiments of $S_1 = 1.00S_0$ and $S_2 = 0.80S_0$, $\alpha_p^1$ is 0.38, $\alpha_p^2$ is 0.36, $\alpha_{pc}^1$ is 0.20, $SWCE_1$ is $-64.0$ W m$^{-2}$, $SWCE_2$ is $-45.1$ W m$^{-2}$. So, the change of the shortwave cloud radiative effect (the left-hand size of Equation 4) is 18.9 W m$^{-2}$, the first term on the right-hand side of Equation 4 is 6.0 W m$^{-2}$, and the second term is 12.6 W m$^{-2}$ (note that the denominator is 3.87 in SAM). In other words, in these two experiments the strength of the shortwave cloud feedback is 6.0 W m$^{-2}$ rather than 18.9 W m$^{-2}$.

**Text S3. Inversion strength indexes**

In literature, there are three indicators that can be used to evaluate the boundary layer inversion strength.

First, the lower tropospheric stability (LTS) is calculated as the difference of potential temperature between surface and 700 hPa (Slingo, 1987):

$$LTS = \theta_{700} - \theta_{sfc}, \tag{5}$$

where $\theta$ is potential temperature.

Second, the estimated inversion strength (EIS) is a more regime-independent predictor of low-level cloud fraction, and it is regarded as the difference of the wet bulb potential temperature between surface and 700 hPa (Wood & Bretherton, 2006):

$$EIS = LTS - \Gamma_m^{850}(z_{700} - LCL), \tag{6}$$

where $\Gamma_m^{850}$ is the moist-adiabatic potential temperature gradient at 850 hPa, $z_{700}$ is the height at 700 hPa, and $LCL$ is the surface-based lifting condensation level.

Third, the estimated cloud-top entrainment index (ECTEI) further considers the humidity gap across the inversion, which can influence the criterion of low-level cloud breakup (Kawai et al., 2017), and it is calculated as:

$$ECTEI = EIS - \beta(L/c_p)(q_{sfc} - q_{700}), \tag{7}$$

where $\beta$ is equal to $(1-k)C_{qgap}$, $k = 0.70$ (MacVean & Mason, 1990), and $C_{qgap} = 0.8$. Besides, $L$ is the latent heat of vapourization of water, $c_p$ is specific heat at constant pressure, and $q$ is specific humidity.

## References

Kawai, H., Koshiro, T., & Webb, M. J. (2017). Interpretation of factors controlling low cloud cover and low cloud feedback using a unified predictive index. *Journal of Climate*, *30*(22), 9119–9131.

MacVean, M., & Mason, P. (1990). Cloud-top entrainment instability through small-scale mixing and its parameterization in numerical models. *Journal of Atmospheric Sciences*, *47*(8), 1012–1030.

Slingo, J. (1987). The development and verification of a cloud prediction scheme for the ECMWF model. *Quarterly Journal of the Royal Meteorological Society*, *113*(477), 899–927.

Wood, R., & Bretherton, C. S. (2006). On the relationship between stratiform low cloud cover and lower-tropospheric stability. *Journal of climate*, *19*(24), 6425–6432.

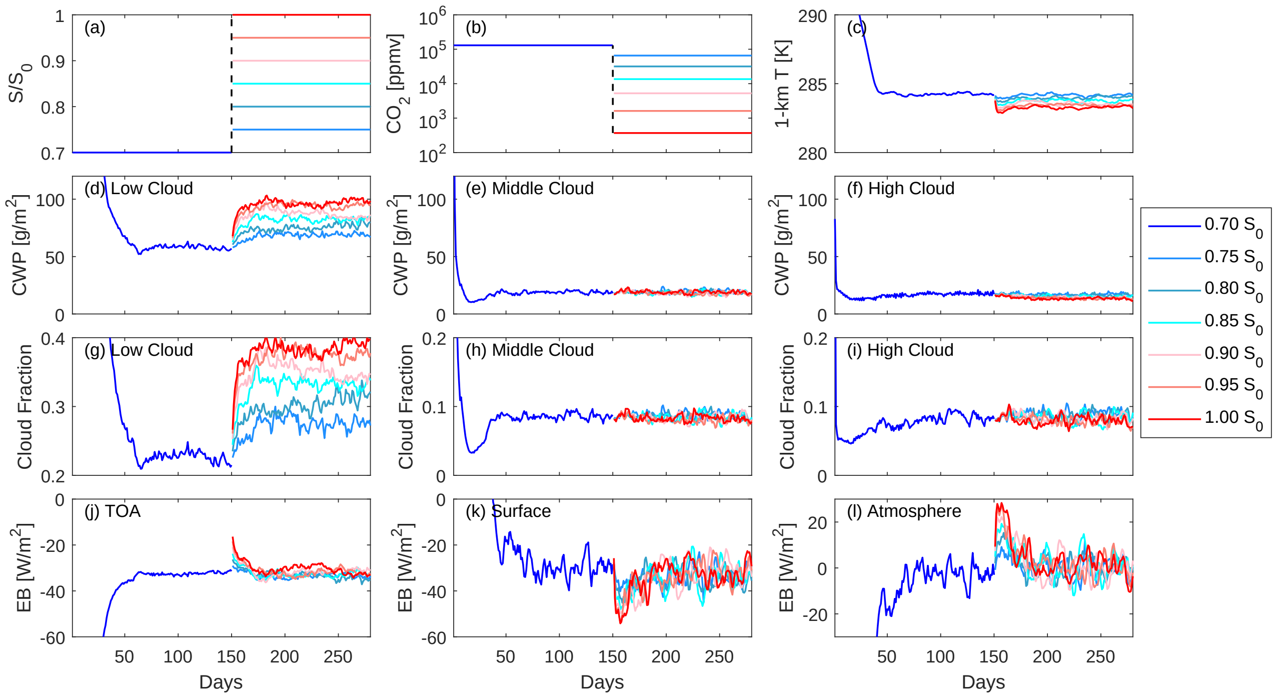


Figure S1: Time-series of (a) solar insolation, (b) $CO_2$ concentration, (c) atmosphere temperature at the level of 1 km, (d)–(f) cloud water paths (CWP) for low-level, middle-level, and high-level clouds, respectively, (g)–(i) same as the panels of (d)–(f) but for cloud fractions, (j)–(k) energy balance (EB) of the TOA and surface, and negative value indicates net downward energy, and (l) energy balance of the atmosphere, and negative value indicates that atmosphere loses energy. The control simulation ($0.70S_0$, blue) was run for 150 model days, and then other simulations were run from its final state for 130 model days. To ensure that all experiments reach equilibrium, we continue running the control simulation to 200 days and find that the climate state remains the same (figure not shown).

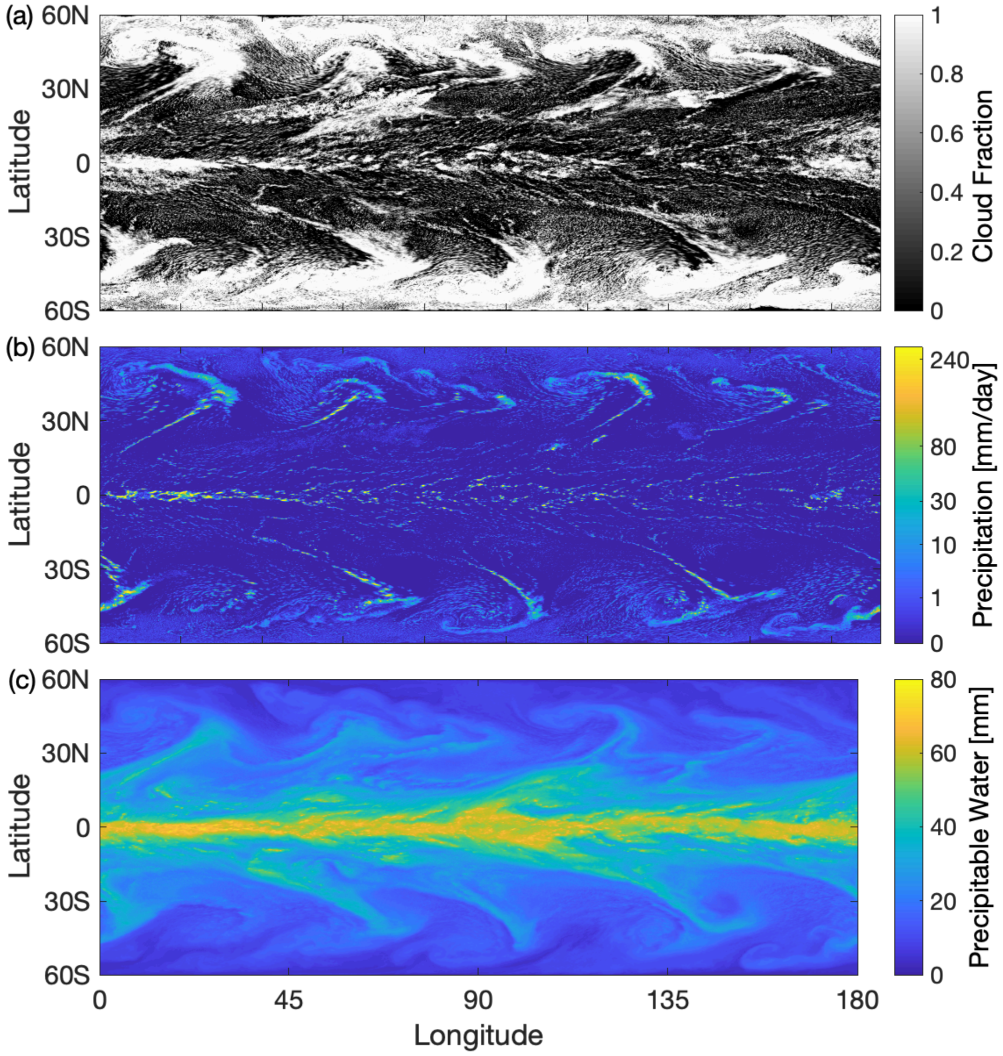


Figure S2: Spatial patterns of hourly-mean (a) cloud fraction, (b) precipitation, and (c) precipitable water in modern Earth simulation (1.00 $S_0$ and 1.04$\times CO_2$).

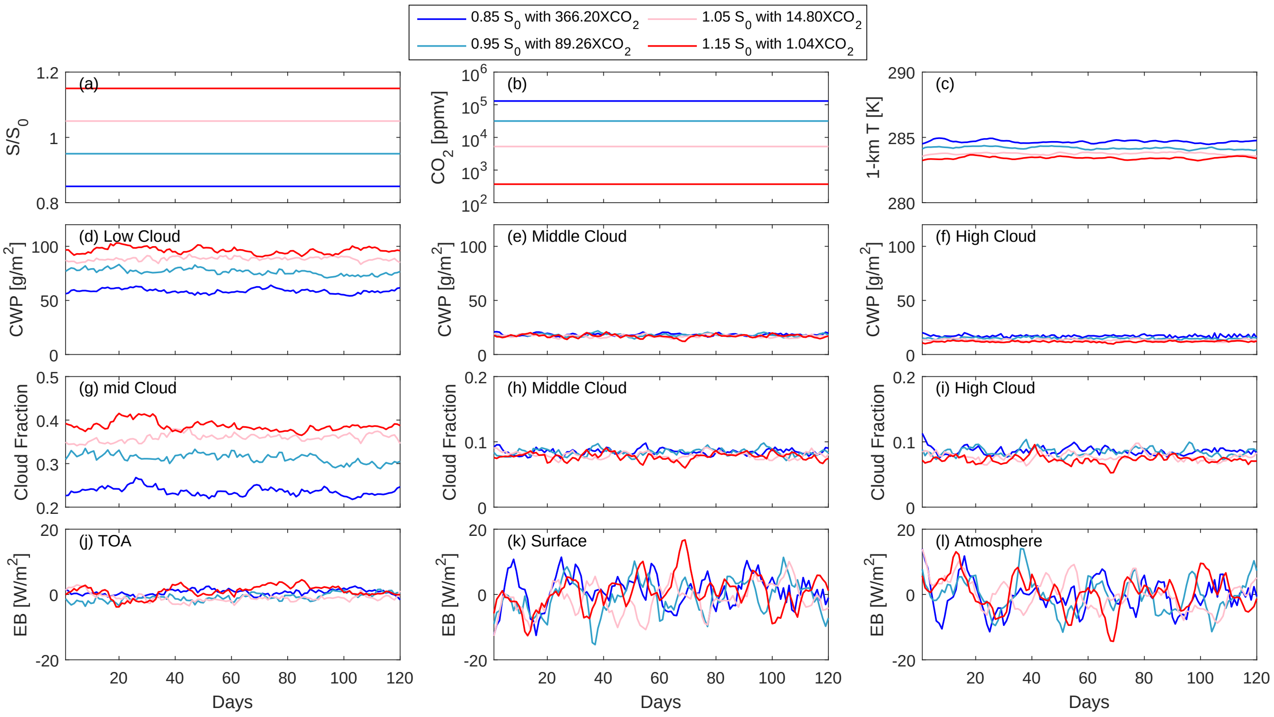


Figure S3: Time-series of the four additional fixed SST simulations. Same as Figure S1, but the TOA and surface are nearly energy-balanced. The solar radiations and $CO_2$ concentrations are 0.85 $S_0$ and 366.20$\times CO_2$, 0.95 $S_0$ and 89.26$\times CO_2$, 1.05 $S_0$ and 14.80$\times CO_2$, and 1.15 $S_0$ and 1.04$\times CO_2$, respectively. These four simulations start from the final states of the 0.70$S_0$, 0.80$S_0$, 0.90$S_0$, and 1.00$S_0$ cases in Figure S1, respectively.

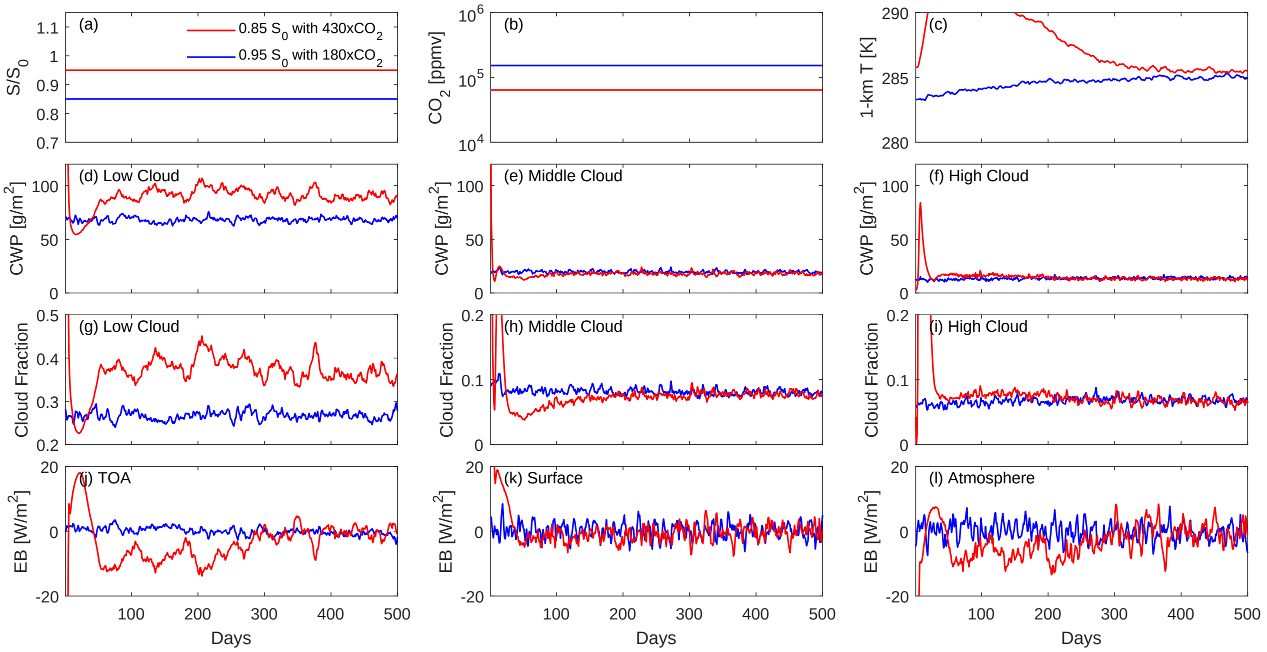


Figure S4: Time-series of slab ocean runs. Same as Figure S1, but for the two slab ocean simulations.

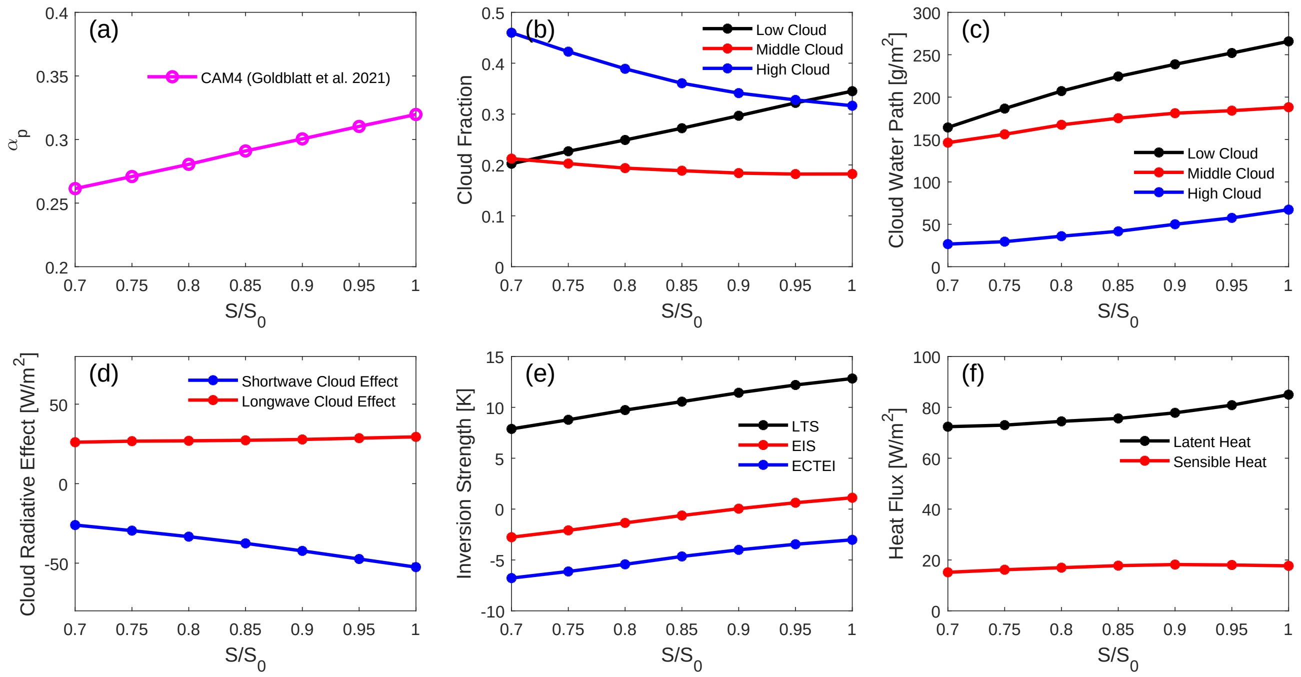


Figure S5: Results of the CAM4 experiments in Goldblatt et al. (2021) under different solar radiations as well as corresponding $CO_2$ concentrations. EIS in (e) is smaller than their Figure 4, because we find an error in their calculations: relative humidity in CAM4 is in percent unit, which means the range of relative humidity is 0 to 100, instead of 0 to 1 used in their calculations.

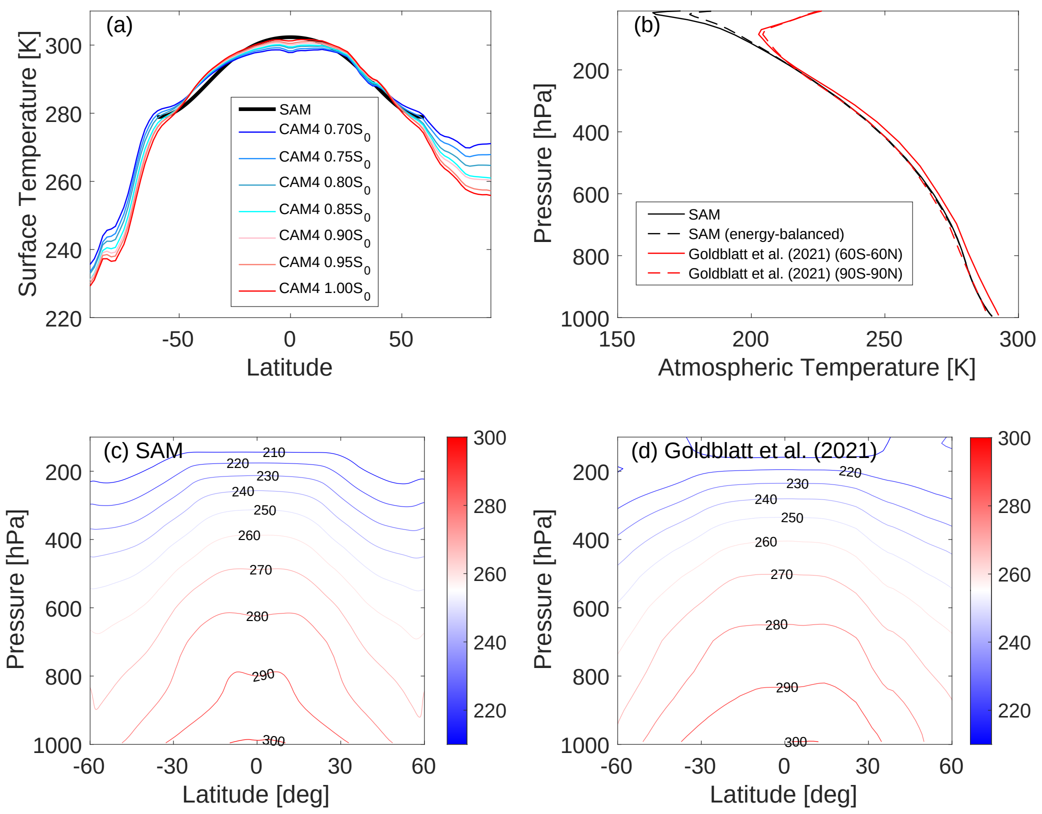


Figure S6: The comparisons of surface and air temperatures between SAM (this study) and CAM4 (Goldblatt et al., 2021). (a) Zonal-mean surface temperature distributions in different runs. (b) Mean temperature profiles in the $1.00S_0$ case. The black solid line represents the fixed SST simulation of 1.00 $S_0$ and $1.04\times CO_2$ (Figure S1), and the black dashed line represents the fixed SST simulation of 1.15 $S_0$ and $1.04\times CO_2$ in which the TOA and surface are nearly energy-balanced (Figure S3). The solid and dashed red lines show the results of CAM4 ($1.00S_0$) averaging over 60°S to 60°N and 90°S to 90°N, respectively. (c) and (d) The comparisons of zonal-mean air temperature ($1.00S_0$).

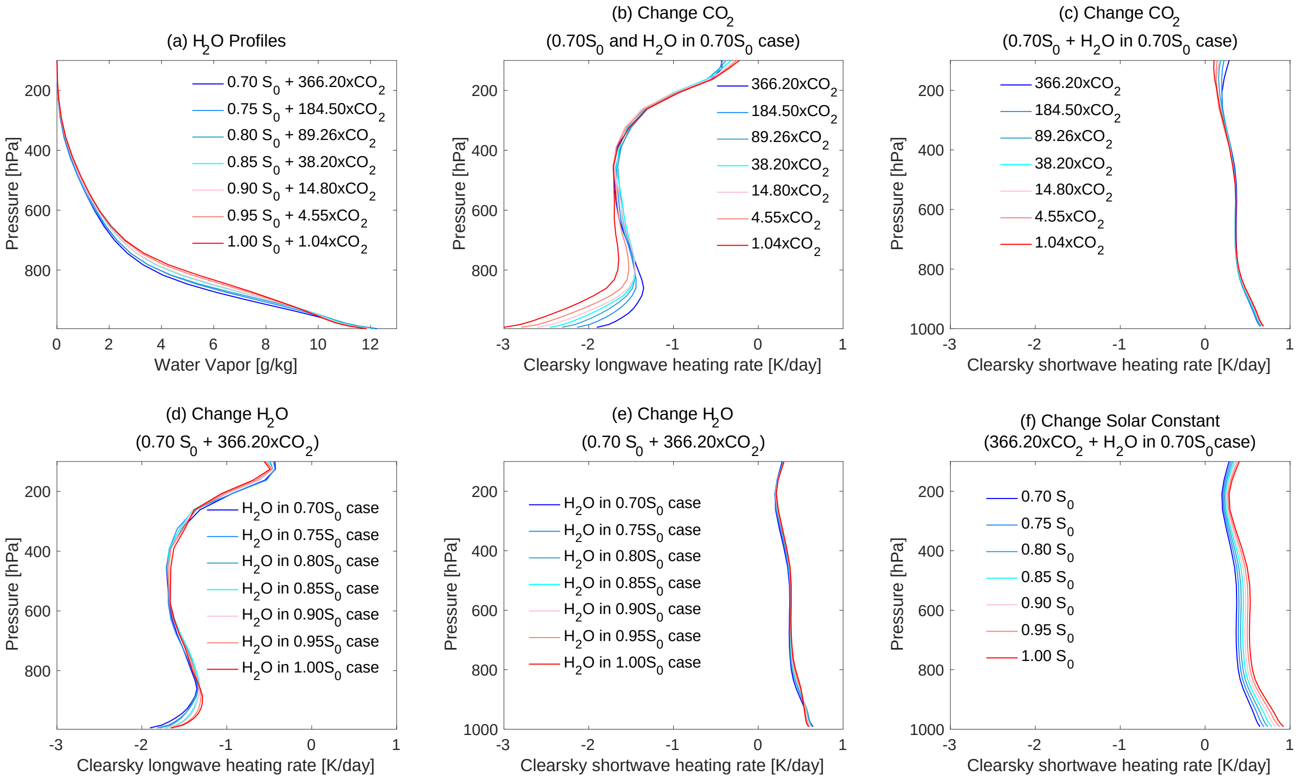


Figure S7: Clearsky radiative heating rates calculated by the 1D radiative-transfer model RRTMG. In all simulations, we use the mean air temperature profile of the control simulation ($0.70S_0$), but change the $CO_2$ concentration, the vertical profile of $H_2O$, or the solar constant. (a) Profiles of water vapor, which are given by the mean value of the last 30 days in the seven simulations of Figure S1. (b)–(c) The influence of $CO_2$ concentration on clear-sky longwave and shortwave heating rates, in which the water vapor profile and solar constant are fixed as the mean values of the control simulation. (d)–(e) The influence of $H_2O$ on clearsky longwave and shortwave heating rates. Here, we use different water vapor profiles as shown in panel (a), but fix the $CO_2$ concentration and solar constant as in the control simulation. (f) The influence of solar constant on clearsky shortwave heating rate. We change solar constant, but fix the $CO_2$ concentration and water vapor profile to be the same as those in the control simulation. For simplicity, we set the volume mixing ratios of $N_2O$, CO, $CH_4$, and $O_2$ to be $10^{-30}$.

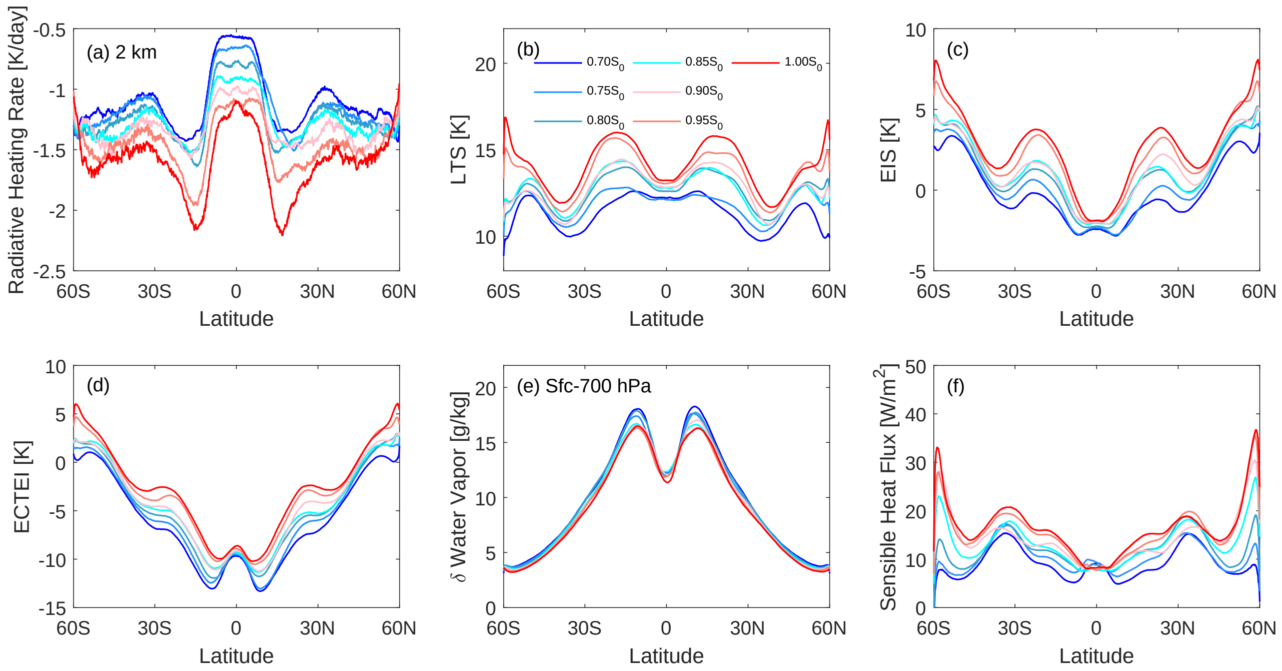


Figure S8: Mechanisms for the low-level cloud feedback. Zonal-mean (a) all-sky radiative heating rate (shortwave plus longwave) at the level of 2 km, (b) lower tropospheric stability (LTS), (c) estimated inversion strength (EIS), (d) estimated cloud-top enrainment index (ECTEI), (e) water vapor difference between the surface and the level of 700 hPa, and (f) surface sensible heat flux. For the definitions of LTS, EIS, and ECTEI, please see Text S3 in this document.

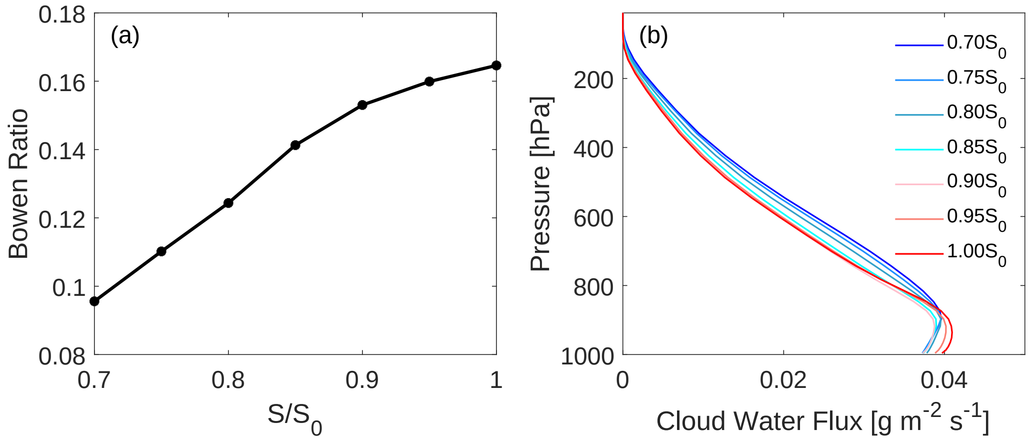


Figure S9: (a) Global-mean Bowen ratios, (b) global-mean profiles of cloud water flux in the SAM experiments shown in Figure S1.

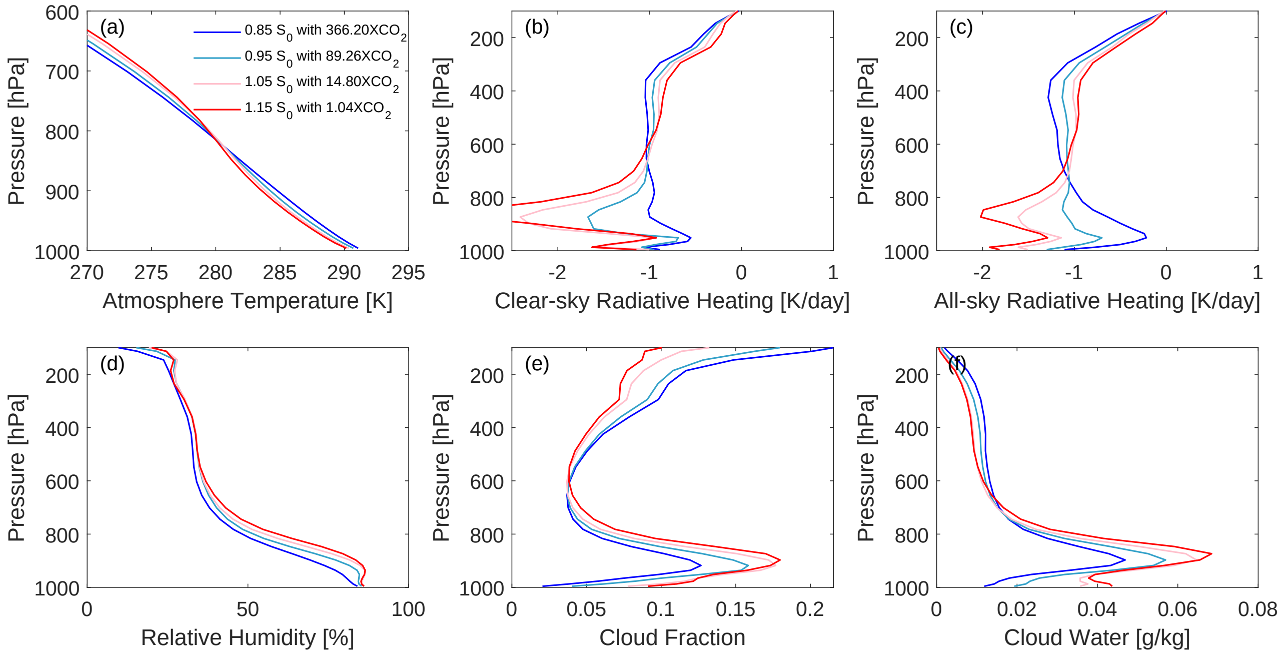


Figure S10: Global-mean profiles of (a) atmosphere temperature (600-1000 hPa), (b) clear-sky radiative heating rate, (c) all-sky radiative heating rate (shortwave plus longwave), (d) relative humidity, (e) cloud fraction, and (f) cloud water, in the four fixed SST experiments shown in Figure S3. The energy budgets for the atmosphere and at the TOA and surface are nearly balanced.

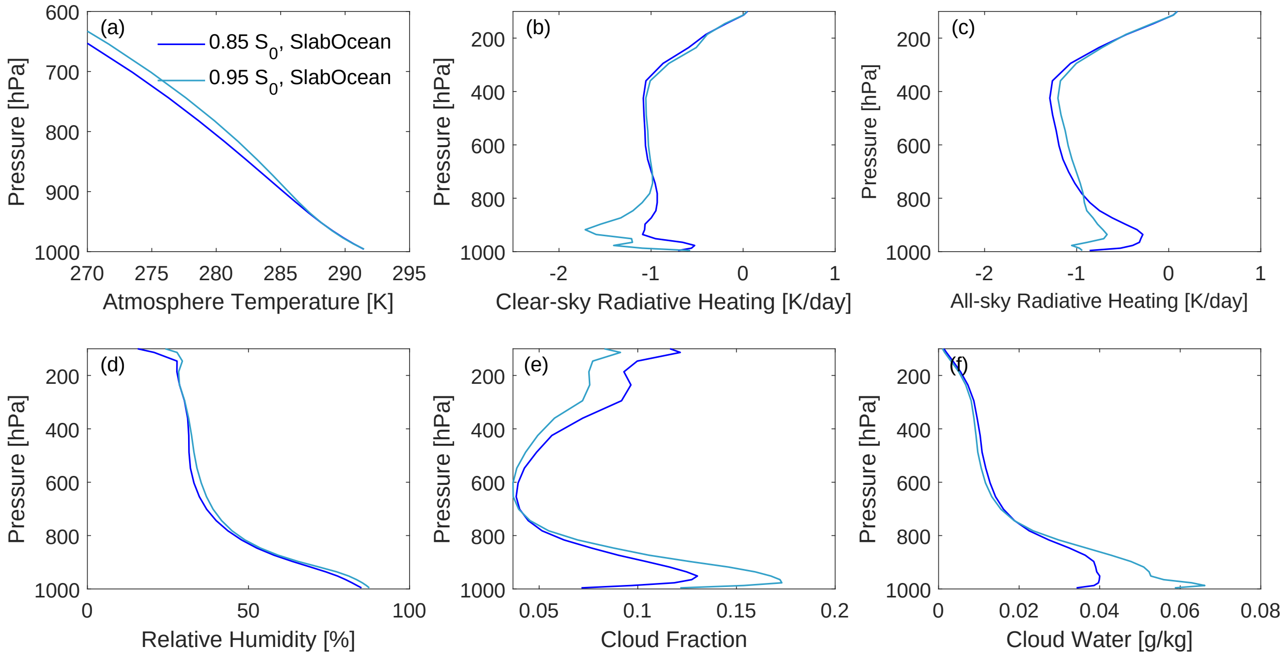


Figure S11: Same as Figure S10, but for the two slab ocean runs.

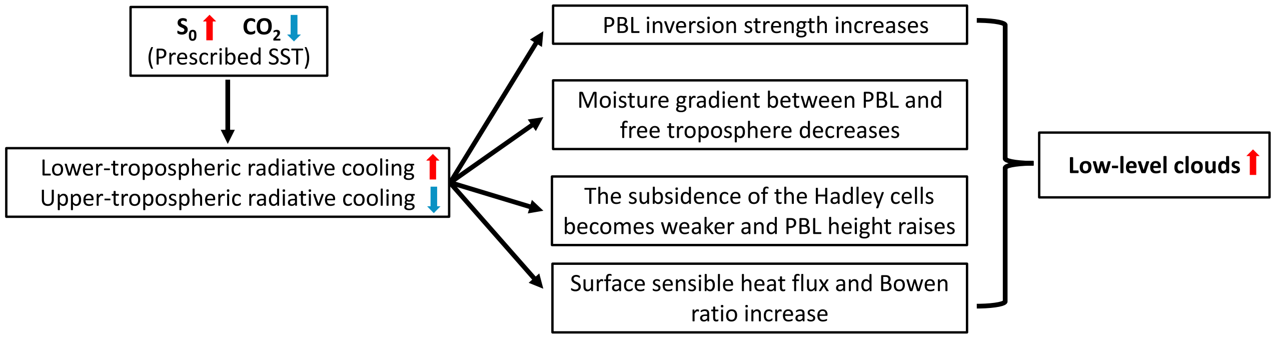


Figure S12: Schematic diagram illustrating the mechanisms of the low-level cloud feedback when the insolation increases but meanwhile $CO_2$ concentration decreases. PBL: planetary boundary layer.
